# Supplementary material for: A Near-Linear Time Approximation Algorithm for Beyond-Worst-Case Graph Clustering
Source: arXiv:2406.04857 source file (2024-06-07)
Supplement: Supplementary file 1 [file appendix.tex]

%\section{Additional tools}\label{section:appendix}

\section{Old proof}

\begin{theorem}\label{theorem:oracle-main}
	Let $n, \alpha> 0\,, \Omega(1)\leq a\leq 1\,, 0< \ell, \leq 1\,,  \Omega(1/\sqrt{\log n})\leq \delta \leq 1/100\,, 0<\rho< 1/\delta\,.$
	Let $G$ be a graph on $\ell \cdot n$ vertices with optimal cut of value at most $\alpha$ that is geometrically expanding up to scale $(\sqrt{\log n}, n)$. 
	
	There exists a $\tilde{O}(\alpha/(n\cdot \ell))$-bounded, $O(\log n)^{100}$-robust, $\Theta(1)$-separation \oracle that, given $G\,, \delta$ and a candidate solution $X$ to \cref{eq:canonical-primal-sdp}, with probability $1-O(\log n)^{-50}$, outputs \textbf{yes} only if it finds a $(a/10)$-balanced cut of value $O(\alpha)$, or if the following conditions hold:
	\begin{enumerate}
		\item[(flatness):] $W:=\Set{i\in [n]\suchthat \Snorm{v_i}>2} \subseteq [n]$  satisfies $\Card{W}< \frac{n}{(\log n)^{100}}$.
		\item[(balance):] $S:= [n]\setminus W$ satisfies $\sum_{i,j \in S} \Snorm{v_i-v_j}\geq 2an$.  
		\item[(flow):] there exists a $a$-balanced partition $(P, P')$ of $V(G)$ satisfying
		\begin{align*}
			\sum_{i \in P\,, j \in P'\,, \ij\in E(G)} \Snorm{v_i-v_j}&\leq O(\alpha)\\
			\Card{E(P, P')}&\leq O(\alpha\cdot \rho)\cdot \sqrt{\log n}\,.
		\end{align*}
		\item [(heavy vertices):] there exists a set of edges $E^*\subseteq E(G)$ of cardinality $O(\alpha/\delta)$ and a partition $(P_1, P_2, V')$ of $V(G)$ such that
		\begin{itemize}
			\item  $\Card{E(P_1, P_2, V')\setminus E^*}\leq O\Paren{ \frac{\alpha}{\delta}\Paren{1+\frac{\ell}{\delta}}}\,.$
			\item $\Abs{\Card{P_1} - \Card{P_2}} \leq an/2$ or $\Card{V'}\geq an/10\,.$
			\item %the optimal $a$-balanced cut on $V'$ has value at most $10\alpha \delta^2$. 
			$\forall \ij \in E(G)\setminus E^*$ with $i,j \in V'$ it holds $\Snorm{v_i-v_j}\leq \delta\,.$
			\item $H_{\delta, n}(X, V')=\emptyset\,.$ 
		\end{itemize}
	\end{enumerate}
	Moreover, if the candidate solution is given in the form of $v_1,\ldots, v_n \in \R^{O(\polylog n)}$ the \oracle  runs in time $\tilde{O}\Paren{\rho\Card{V(G)}^{1+O(1/\rho^2)}+\rho\Card{E(G)}^{1+O(1/\rho^2)}}$ and finds the set $E^*$ and the partitions $(P_1, P_2, V')$ and $(P,P')$.
	Finally, in the \textbf{no} case  the resulting feedback matrix has $O(m+n)$ non-zero entries.
\end{theorem}

As already mention the crucial consequence of geometric expansion of the input graph is that the removal procedure in steps $(c)\,, (d)$ significantly decreases the optimal objective value of the program over the remaining vertices. 
We can finally prove the Theorem.

\begin{proof}[Proof of \cref{theorem:balanced-cut-main-technical}]
	We set $T=\Theta(\sqrt{\log n})$. Notice that  the running time of the oracle and thus by \cref{lemma:fast-computation-approx-mmw} also the  running time of \cref{algorithm:approx-mmw} are both bounded by 
	$\tilde{O}\Paren{\rho\Card{V(G)}^{1+O(1/\rho^2)}+\rho\Card{E(G)}^{1+O(1/\rho^2)}}$. So overall \cref{algorithm:balanced-cut} runs in the desired time.
	%We use $\super{T}{i}$ to denote the numer of iterations of \cref{algorithm:mmw} in each iteration of \cref{algorithm:balanced-cut}.
	
	Now by \cref{lemma:robust-oracle} and the bounded width in \cref{theorem:oracle-main}, with high probability during each iteration $i$ of \cref{algorithm:balanced-cut}, the \oracle  outputs \textbf{no} at most $O(\log n)^{10}$ times.

	Hence consider a fixed iteration $i$, we assume $\super{\alpha}{0}=\alpha\,, \super{\ell}{0}=1$ and $\super{\delta}{0}=1/(100\rho)$. Let $\super{\alpha}{i}$ be the cost of the minimum feasible solution on the remaining graph $\super{G}{i}$ on $\super{\ell}{i}\cdot n$ vertices. Let $\super{\delta}{i}$ be the current value of $\delta$. Let $\super{E}{i}$ be the set of edges removed at iteration $i$ and $(\super{P}{i}_1, \super{P}{i}_2, \super{V'}{i})$ the partition at iteration $i$.
	Notice that if  at some point $\super{\alpha}{i}\leq \frac{O(1))}{\sqrt{\log n}}\cdot (n^2\cdot \eta)\leq O(\alpha/\log n)$ then we simply return a $O(\sqrt{\log n})$-approximation of the optimum balanced cut as in the last step of \cref{algorithm:balanced-cut}, yielding an $(a/10)$-balanced cut of value at most $O(n^2\cdot \eta)$ for the remaining graph.
	
	So we may assume at the current iteration $i$, $\super{\alpha}{i}\geq \omega\Paren{1/\log n} \cdot (n^2\cdot \eta)$. 
	%Now the result follows by showing that first, at each step, removing vertices in $\super{P}{i}_1$ and $\super{P}{i}_2$ we cut at most $O\Paren{\frac{\super{\alpha}{i}}{\super{\delta}{i}}\Paren{1+\frac{\super{\ell}{i}}{\super{\delta}{i}}}}$ edges. Second that $\super{\alpha}{i}\leq 10\cdot \super{\alpha}{i-1}\cdot \Paren{\super{\delta}{i-1}}^2$.
	Now the result follows by showing that, at each step, it holds
	\begin{align}\label{eq:geometric-expansion}
		\super{\alpha}{i}\leq 10\cdot \super{\alpha}{i-1}\cdot \Paren{\super{\delta}{i-1}}^2\,.
	\end{align} 
	Indeed suppose the claim holds. By construction all the edges in the final cut are in
	\begin{align*}
		\Paren{\underset{i\leq T}{\bigcup} \super{E}{i}} \cup \Paren{\underset{i\leq T}{\bigcup} E(\super{P}{i}_1, \super{P}{i}_2, \super{V'}{i})\setminus \super{E}{i}}\,.
	\end{align*}
	By \cref{eq:geometric-expansion} we can bound the first term as
	\begin{align*}
		\Card{\underset{i\leq T}{\bigcup} \super{E}{i}}\leq O(\alpha\cdot \rho)\,.
	\end{align*}
	For the second term we have
	\begin{align*}
		\Card{\underset{i\leq T}{\bigcup} E(\super{P}{i}_1, \super{P}{i}_2, \super{V'}{i})}&\leq 
		\sum_{i\leq T} O\Paren{\frac{\super{\alpha}{i}}{\super{\delta}{i}}\Paren{1+\frac{\super{\ell}{i}}{\super{\delta}{i}}}} \\
		&\leq O\Paren{\sum_{i\leq T} \frac{\super{\alpha}{i}}{\super{\delta}{i} } + \frac{\super{\alpha}{i}\cdot \super{\ell}{i}}{\Paren{\super{\delta}{i}}^2}}\\
		&\leq O\Paren{\sum_{i\leq T}\super{\alpha}{i}\cdot \Paren{\super{\delta}{i}+\super{\ell}{i+1}}}\\
		&\leq O\Paren{\sum_{i\leq T}\super{\alpha}{i}\cdot \Paren{\super{\delta}{i}+\super{\ell}{i}}}\\
		&\leq \alpha\cdot O\Paren{\sum_{i\leq T} \super{\delta}{i}+\super{\ell}{i}}\\
		&\leq O(\alpha)\,,
	\end{align*}
	where in the second step we used the inequalities
	\begin{align*}
		\frac{\super{\alpha}{i}}{\super{\delta}{i}}&\leq 10^3\cdot \super{\alpha}{i-1}\cdot \super{\delta}{i-1}\,,\\
		\frac{\super{\alpha}{i}\cdot \super{\ell}{i}}{\Paren{\super{\delta}{i}}^2}&\leq  10^5\cdot \super{\alpha}{i-1}\cdot \super{\ell}{{i}}\,,
	\end{align*}
	both following from \cref{eq:geometric-expansion}.
	Thus it remains to prove \cref{eq:geometric-expansion}.
	At each iteration $i$, the set $V(\super{G}{i})$ does not contain edges of length more than $\super{\delta}{i}$ in the embedding as well as $(\super{\delta}{i}, n)$ heavy vertices. Thus by \cref{theorem:geometric-expansion-random-graphs}, with probability at least $1- n^{-\Omega(1)}$, the set $V(\super{G}{i})$ is geometrically expanding with cut value $O(\super{\alpha}{i})$ at scale $(\super{\delta}{i}, n)$. Then \cref{eq:geometric-expansion} follows as desired.
	
	Finally, we remark that if \cref{eq:geometric-expansion} is not satisfied then
	we have 
	\begin{align*}
		\Paren{\underset{i\leq T}{\bigcup} \super{E}{i}} \cup \Paren{\underset{i\leq T}{\bigcup} E(\super{P}{i}_1, \super{P}{i}_2, \super{V'}{i})\setminus \super{E}{i}}&\leq O(\alpha)\cdot\Paren{\sum_{i\leq T}\frac{1}{\super{\delta}{i}}}\\
		&\leq O(\alpha \cdot \rho \cdot \sqrt{\log n})\,.
	\end{align*}
	That is, without geometric expansion the algorithm provides a $a/10$-balanced cut of cardinality $O(\alpha\rho\sqrt{\log n})$.
	%Thus for the first point, notice that at each iteration we have $\Card{E(P_1, P_2, V')\setminus \super{E}{i}}\leq O\Paren{ \frac{\alpha}{\delta}\Paren{1+\frac{\ell}{\delta}}}$, which means that removing $P_1$ and $P_2$ we cut at most that number of edges. 
	%For the second point, with probability at least $1- n^{-\Omega(1)}$, by \cref{theorem:geometric-expansion-random-graphs} the set $V(\super{G}{i})$ is geometrically expanding with cut value $O(\super{\alpha}{i})$ at scale $(\super{\delta}{i}, n)$. Thus it follows that $\super{\alpha}{i+1}\leq 10\cdot  \Paren{\super{\delta}{i}}^2\cdot \super{\alpha}{i}$ as desired.
\end{proof}

\section{Missing proofs}\label{section:missing-proofs}

We explain here how one can obtain the statement in \cref{lemma:flow-oracle} from \cite{DBLP:conf-focs-Sherman09}:
\begin{quote}
	\textit{Furthermore, the oracle outputs \textbf{no} with probability at least $1-O(\log n)^{-100}$ over random bits if
	\begin{align}\label{eq:bound-delta-edges}
		\Card{\Set{\ij \in V(G)\suchthat \Snorm{v_i-v_j}\geq \delta} }\geq O\Paren{\frac{\alpha}{\delta}}\,.
	\end{align}}
\end{quote}

Recall that the oracle in \cite{DBLP:conf-focs-Sherman09} runs the  following algorithm a predefined number of times.

\begin{algorithmbox}[Flow or cut, \cite{DBLP:conf-stoc-AroraK07}]\label{algorithm:flow-or-cut}
	\mbox{}\\
	\textbf{Input:} A graph $G$, a candidate solution $X$ to \cref{eq:extended-balanced-cut-primal-sdp} satisfying the flatness and balance conditions in \cref{lemma:basic-oracle}. Set $S\subseteq [n]$ as in \cref{lemma:basic-oracle}, $d=O\Paren{\frac{\alpha}{\Card{V(G)}}\log n}$, $\sigma \geq \Omega(a)$, $T >0$. 
	
	\noindent
	Repeat $T$ times:
	\begin{enumerate}
		\item Pick $\mathbf{u}\sim N(0, \Id)$. Let $m$ be the median values of the products $\iprod{v_i, \mathbf{u}}$ for $i\in S$. 
		\item By a linear scan [Appendix B, \cite{DBLP:conf-stoc-AroraK07}] find sets $P_\mathbf{u}, P'_\mathbf{u}\subseteq S$ of size at least $\Omega(an)$ such that for all $i\in P_\mathbf{u}\,, j\in P'_\mathbf{u}$ we have $\iprod{v_j-v_i, \mathbf{u}}\geq \sigma$.
		\item If such sets $P_\mathbf{u}, P'_\mathbf{u}$ exist, connect all nodes of $P_\mathbf{u}$ to (an artificial) source with edges of capacity $d$, and connect all nodes of $P'_\mathbf{u}$ to (an artificial) sink with edges of capacity $d$.
		\item Compute the maximum flow over the partition: $\sum_{i \in P_\mathbf{u}\,, j \in P'_\mathbf{u}}f_\ij$. If the min-cut is at most $O(\alpha)$, return the cut. Else store  the flow.%$\sum_{i \in P_\mathbf{u}\,, j \in P'_\mathbf{u}}f_\ij\Snorm{v_i-v_j}$. 
	\end{enumerate}
	Return the maximum flow found.
\end{algorithmbox}

Consider the parameters of \cref{lemma:flow-oracle}. We run \cref{algorithm:flow-or-cut} $T=\Theta(\log n)^{100}$ times.
Using the Gaussian nature of projections, with very high probability, we obtain sets $P_{\mathbf{u}}\,, P'_{\mathbf{u}}$ of size $\Omega(an)$. Moreover the probability that an edge $uv\in E(G)$ with $\Snorm{u-v}\geq \delta$ has only one endpoint in $P_{\mathbf{u}}$ is at least $C\cdot\delta$ for some fixed constant $C>0$.

Compute the maximum $d$-regular $(P_{\mathbf{u}}, P'_{\mathbf{u}})$ flow, where $d=O\Paren{\frac{a\cdot \alpha\cdot \log n}{n}}$ (this involves the entire graph $G$, not just nodes in $S$). 
Suppose the total flow obtained is at least $C' \cdot \alpha/\delta$ for some large enough fixed constant $C'>0$. Then if \cref{eq:bound-delta-edges} holds we have 
\begin{align*}
	\sum_{i \in P_{\mathbf{u}}\,, j \in P'_{\mathbf{u}}} f_\ij \Snorm{v_i-v_j} \geq C\cdot \alpha\,.
\end{align*}

%for any pair of nodes $i\,, j$, we have that $\Abs{\iprod{v_i-v_j, u}}\leq O(\log n)\Snorm{v_i-v_j}\,.$
Thus, we conclude that with constant probability we obtain sets $P_{\mathbf{u}}\,, P'_{\mathbf{u}}$ such that $\forall i \in P_{\mathbf{u}}$ and $\forall j \in P'_{\mathbf{u}}$, we have $\Snorm{v_i - v_j}\geq C/\log n$ for some fixed constant $C>0$.
Assuming this is the case, we compute the maximum $d$-regular $(P_{\mathbf{u}}, P'_{\mathbf{u}})$ flow, where $d=O\Paren{\frac{a\cdot \alpha\cdot \log n}{n}}$ (this involves the entire graph $G$, not just nodes in $S$). 
Suppose the total flow obtained is at least $C' \cdot \alpha/\delta$ for some large enough fixed constant $C'>0$. Then if \cref{eq:bound-delta-edges} holds we have 
\begin{align*}
	\sum_{i \in P_{\mathbf{u}}\,, j \in P'_{\mathbf{u}}} f_\ij \Snorm{v_i-v_j} \geq C\cdot \alpha\,.
\end{align*}
Let $F$ to be the Laplacian of the weighted graph corresponding to the flow and let $D$ be the Laplacian of the complete weighted graph where only edges $\ij$ with $i \in P_\mathbf{u}$ and $j \in P_\mathbf{u}$ have weight $f_\ij$, and the rest have $0$ weight.  By definition 
\begin{align*}
	\iprod{D, X} = \sum_{i \in P_{\mathbf{u}}\,, j \in P'_{\mathbf{u}}} f_\ij \Snorm{v_i-v_j}
\end{align*}
and  $\sum_p f_p T_p= F-D\,.$
Thus we set $x_i=\alpha/n$ for all $i \in V(G)$, $f_p$ as in the computed flow for all $p$ and all other variables to $0$. The feedback matrix $Y$ becomes $\frac{\alpha}{n}\Id+F-D-F=\frac{\alpha}{n}\Id-D$ and we have
\begin{align*}
	\iprod{\frac{\alpha}{\Card{V(G)}}\Id-D, X}\leq \alpha - O(\alpha) <  -\alpha<0\,.
\end{align*}
Moreover notice that $\Norm{\frac{\alpha}{n}\Id-D}\leq O\Paren{\frac{\alpha}{n}}+d\leq \tilde{O}\Paren{\frac{\alpha}{n}}\,.$
In conclusion, in this case the \oracle finds a separating hyperplane and outputs \textbf{no}.

Conversely suppose the flow is smaller than $C' \cdot \alpha \cdot \log n$. By the max-flow-min-cut theorem, the cut obtained is also at most this size. Moreover, by choice of $d$ this cut must be $a/2$-balanced.
\Tnote{Improve the paragraph below}
Finally, to argue that with  probability at least $1-O(\log n)^{-200}$ we have
\begin{align}\label{eq:few-long-edges}
	\Card{\Set{\ij \in V(G)\suchthat \Snorm{v_i-v_j}\geq \delta} }\leq O\Paren{\frac{\alpha+\gamma}{\delta}}\,,
\end{align}
we simply run \cref{algorithm:flow-or-cut} $O(\log n)^{200}$ times. Indeed at each trial we either find a feedback matrix or a direction $\frac{u}{\Norm{u}}\in \mathbb{S}^n$ for which \cref{algorithm:flow-or-cut} returns a partition $(P_{\mathbf{u}},P'_{\mathbf{u}})$ of $V(G)$ satisfying
\begin{align*}
	\sum_{i \in P_{\mathbf{u}}\,, j \in P'_{\mathbf{u}}}f_\ij \Snorm{v_i-v_j}\leq O(\alpha+\gamma)\,.
\end{align*}
As for a $1-O(\log n)^{-200}$ fraction of directions in $ \mathbb{S}^n$ we obtain this result, the claim follows.
\Tnote{Double check running time}
For the running time, to compute the update we may use the pseudo-decomposition of flows as in \cite{DBLP:conf-focs-Sherman09} and the max flow algorithm of \cref{theorem:max-flow-linear-time}.

We can now prove the Lemma.

\begin{proof}[Proof sketch of \cref{lemma:flow-oracle}]
	We run \cref{algorithm:flow-or-cut}.
	Using the Gaussian nature of projections, with very high probability, for any pair of nodes $i\,, j$, we have that $\Abs{\iprod{v_i-v_j, u}}\leq O(\log n)\Snorm{v_i-v_j}\,.$
	Thus, we conclude that with constant probability we obtain sets $P_{\mathbf{u}}\,, P'_{\mathbf{u}}$ such that $\forall i \in P_{\mathbf{u}}$ and $\forall j \in P'_{\mathbf{u}}$, we have $\Snorm{v_i - v_j}\geq C/\log n$ for some fixed constant $C>0$.
	Assuming this is the case, we compute the maximum $d$-regular $(P_{\mathbf{u}}, P'_{\mathbf{u}})$ flow, where $d=O\Paren{\frac{a\cdot \alpha\cdot \log n}{n}}$ (this involves the entire graph $G$, not just nodes in $S$). 
	Suppose the total flow obtained is at least $C' \cdot \alpha \cdot \log n$ for some large enough fixed constant $C'>0$. Then we have
	\begin{align*}
		\sum_{i \in P_{\mathbf{u}}\,, j \in P'_{\mathbf{u}}} f_\ij \Snorm{v_i-v_j} \geq \Omega(\alpha)\,.
	\end{align*}
	Let $F$ to be the Laplacian of the weighted graph corresponding to the flow and let $D$ be the Laplacian of the complete weighted graph where only edges $\ij$ with $i \in P_\mathbf{u}$ and $j \in P_\mathbf{u}$ have weight $f_\ij$, and the rest have $0$ weight.  By definition 
	\begin{align*}
		\iprod{D, X} = \sum_{i \in P_{\mathbf{u}}\,, j \in P'_{\mathbf{u}}} f_\ij \Snorm{v_i-v_j}
	\end{align*}
	and  $\sum_p f_p T_p= F-D\,.$
	Thus we set $x_i=\alpha/n$ for all $i \in V(G)$, $f_p$ as in the computed flow for all $p$ and all other variables to $0$. The feedback matrix $Y$ becomes $\frac{\alpha}{n}\Id+F-D-F=\frac{\alpha}{n}\Id-D$ and we have
	\begin{align*}
		\iprod{\frac{\alpha}{\Card{V(G)}}\Id-D, X}\leq \alpha - O(\alpha) <  -\alpha<0\,.
	\end{align*}
	Moreover notice that $\Norm{\frac{\alpha}{n}\Id-D}\leq O\Paren{\frac{\alpha}{n}}+d\leq \tilde{O}\Paren{\frac{\alpha}{n}}\,.$
	In conclusion, in this case the \oracle finds a separating hyperplane and outputs \textbf{no}.
	
	Conversely suppose the flow is smaller than $C' \cdot \alpha \cdot \log n$. By the max-flow-min-cut theorem, the cut obtained is also at most this size. Moreover, by choice of $d$ this cut must be $a/2$-balanced.
	\Tnote{Improve the paragraph below}
	Finally, to argue that with  probability at least $1-O(\log n)^{-200}$ we have
	\begin{align}\label{eq:few-long-edges}
		\Card{\Set{\ij \in V(G)\suchthat \Snorm{v_i-v_j}\geq \delta} }\leq O\Paren{\frac{\alpha+\gamma}{\delta}}\,,
	\end{align}
	we simply run \cref{algorithm:flow-or-cut} $O(\log n)^{200}$ times. Indeed at each trial we either find a feedback matrix or a direction $\frac{u}{\Norm{u}}\in \mathbb{S}^n$ for which \cref{algorithm:flow-or-cut} returns a partition $(P_{\mathbf{u}},P'_{\mathbf{u}})$ of $V(G)$ satisfying
	\begin{align*}
		\sum_{i \in P_{\mathbf{u}}\,, j \in P'_{\mathbf{u}}}f_\ij \Snorm{v_i-v_j}\leq O(\alpha+\gamma)\,.
	\end{align*}
	As for a $1-O(\log n)^{-200}$ fraction of directions in $ \mathbb{S}^n$ we obtain this result, the claim follows.
	\Tnote{Double check running time}
	For the running time, to compute the update we may use the pseudo-decomposition of flows as in \cite{DBLP:conf-focs-Sherman09} and the max flow algorithm of \cref{theorem:max-flow-linear-time}.
\end{proof}

% MAtrix multiplicative weights proof

For later convenience we include a proof.
The proof of the theorem relies on a result --at the heart of 
the matrix multiplicative weights method-- which amounts to an upper bound the largest eigenvalue of a sum of symmetric matrices.

\begin{theorem}[\cite{DBLP:conf-stoc-AroraK07, DBLP:conf-soda-Steurer10}]\label{theorem:mmw-eigenvalue-bound}
	Let $\epsilon>0$ be small enough and let $\super{Y}{1},\ldots,\super{Y}{T}$ be a sequence in $\cS_n$ with $0\sle \super{Y}{t}\sle \Id_n$, for all $t\in [T]$. Then
	\begin{align*}
		\lambda_{\max}\Paren{\sum_{t\in [T]} \super{Y}{t}} < (1+\eps)\sum_{t\in [T]} \iprod{\super{Y}{t}, \super{X}{t}} + \tfrac{\log n}{\eps}\,,
	\end{align*}
	where $\super{X}{t} = \exp\Paren{\eps\sum_{t'<t}Y_{t'}}/\Tr\Paren{\eps\sum_{t'<t}Y_{t'}}$.
	\begin{proof}
		We start with the following chain of inequalities
		\begin{align*}
			\exp\Paren{\eps\lambda_{\max}\Paren{\sum_{t\in [T]}\super{Y}{t}}}&\leq\Tr\exp\Paren{\eps\sum_{t\in [T]}\super{Y}{t}}\\
			&\leq \Tr\Brac{\exp\Paren{\eps\sum_{t\in [T-1]}\super{Y}{t}}\cdot \exp\Paren{\eps \super{Y}{T}}}\\
			&\leq  \Tr\Brac{\exp\Paren{\eps\sum_{t\in [T-1]}\super{Y}{t}}\cdot \Paren{\Id_n+\Paren{e^\eps-1}\super{Y}{T}}}\\
			&=\Tr\Brac{\exp\Paren{\eps\sum_{t\in [T-1]}\super{Y}{t}}}\Paren{1+\Paren{e^\eps-1}\iprod{\super{X}{T}, \super{Y}{T}}}\\
			&\leq \Tr\Brac{\exp\Paren{\eps\sum_{t\in [T-1]}\super{Y}{t}}}\exp\Paren{(e^\eps-1)\iprod{\super{X}{T}, \super{Y}{T}}}\,.
		\end{align*}
		Here in the second step we used the Golden-Thompson inequality \cite{golden1965lower, thompson1965inequality} $\Tr\exp(A+B)\leq \Tr\exp(A)\Tr\exp(B)$. In the third step we used the fact that  $(1-\eta)^{A}\sle (\Id-\eta A)$ for $0\sle A\sle \Id_n$ and $\eta>0$.
		Repeating the argument for all $t\in [T]$ we get
		\begin{align*}
			\exp\Paren{\eps\lambda_{\max}\Paren{\sum_{t\in [T]}\super{Y}{t}}}&\leq \exp\Paren{\Paren{e^\eps-1}\sum_{t\in [T]}\iprod{\super{Y}{t}, \super{X}{t}}\cdot n}\,.
		\end{align*}
		Finally, the result follows noticing that $e^\eps-1<\eps+\eps^2$, for small enough $\epsilon$.
	\end{proof}
\end{theorem}

We can use \cref{theorem:mmw-eigenvalue-bound} to obtain the desired algorithmic result.

\begin{proof}[Proof of \cref{theorem:result-mmw}]
	We prove the argument by contradiction. We may rescale the program so that $\alpha=1$ and any feasible solution is in $\Delta_n(r/\alpha)$. Thus let $X'$ be a feasible solution to the program with objective value $1$. Applying \cref{theorem:mmw-eigenvalue-bound}, for $\super{Z}{t} = \frac{1}{2}\super{Y}{t}+\frac{1}{2}\Id_n$ we get
	\begin{align*}
		\frac{\alpha}{r}\iprod{X', \sum_{t\in [T]}\super{Z}{t}} &\leq  \lambda_{\max}\Paren{\sum_{t\in [T]}\super{Z}{t}}\\
		&< \frac{\alpha(1+\eps)}{r}\sum_{t\in [T]}\iprod{\super{Z}{t}, \super{X}{t}}+\frac{\log n}{\eps}\\
		&=\frac{\alpha(1+\eps)}{2r}\sum_{t\in [T]}\iprod{\super{Y}{t}, \super{X}{t}}+\frac{\alpha(1+\eps)}{2r}\sum_{t\in [T]}\iprod{\Id_n, \super{X}{t} }+\frac{\log n}{\eps}
	\end{align*}
	This implies
	\begin{align*}
		\frac{\alpha}{r}\iprod{X', \sum_{t\in [T]}\super{Y}{t}} &< - \frac{\alpha}{r}\iprod{M, \frac{T}{2}\Id_n} + \frac{\alpha(1+\eps)}{r}\sum_{t\in [T]}\iprod{\super{Y}{t}, \super{X}{t}}+\frac{\alpha(1+\eps)}{r}\sum_{t\in [T]}\iprod{\Id_n, \super{X}{t} }+\frac{2\log n}{\eps}\\
		& = \frac{\alpha(1+\eps)}{r}\sum_{t\in [T]}\iprod{\super{Y}{t}, \super{X}{t}} + \frac{2\log n}{\eps} + T\eps\,.
	\end{align*}
	On the other hand, since the \oracle always returned \textbf{no}, by choice of $X'$
	\begin{align*}
		\sum_{t\in [T]}\iprod{X'-(1+\eps)\super{X}{t}, \super{Y}{t}}\geq \tfrac{\gamma}{\rho} T \geq \frac{2r\eps}{\alpha} T\,.
	\end{align*}
	Putting the two together
	\begin{align*}
		\frac{2r\eps}{\alpha} T\leq \frac{2r\log n}{\alpha\eps} + \frac{r\eps}{\alpha}T\,.
	\end{align*}
	This contradicts the premise $T\geq \frac{2\log n}{\eps^2}$.
\end{proof}
